# Supplementary material for: Controlling Coherent Quantum Dot Interactions
Source: arXiv:1705.04730 source file (2017-10-13)
Supplement: Supplementary file 1 [file Supplement.pdf]

# Supplemental Material for
# "Controlling Coherent Quantum Dot Interactions"

Eric W. Martin and Steven T. Cundiff*
*Applied Physics Program and Department of Physics University of Michigan,*
*Ann Arbor, MI 48109-1040, USA*

(Dated: October 12, 2017)

## EXPERIMENTAL SETUP

We use a variety of coherent pulse sequences to probe the quantum dot sample. Each multidimensional coherent spectroscopy (MDCS) sequence is defined by pulse and pulse conjugate ordering. Each are used to either emphasize or excite different resonances in the sample [1, 2]. As discussed in the paper and in technical papers describing collinear MDCS [3, 4], the signal resulting from each pulse sequence can be isolated by first tagging each pulse using an acousto-optic modulator (AOM) to shift its frequency, and then detecting the modulated four-wave-mixing signal at a defined frequency. A diagram describing the setup is shown in Figure 1. In order to sample the fluctuations and generate a phase stabilizing reference, we copropagate the MDCS beams with a continuous-wave (CW) diode laser tuned to 762 nm (1627 meV). Other collinear MDCS techniques excite samples with four pulses and measure a population signal like photocurrent or photoluminescence. The way in which our implementation differs is that we induce a radiating four wave mixing signal with three pulses and interfere that field with a local oscillator on an amplified photodetector. In order to sample all the path length fluctuations it is therefore uniquely necessary that a CW beam copropagate one of the beams to the sample and to the combination of the signal with the local oscillator. To not generate a signal of its own or be given a nonlinear phase, it is important that this beam not interact with the sample. We thus keep the CW that reflects off the sample at a very low intensity ($< 50$ nW) and red detuned from all sample resonances by 14 meV.

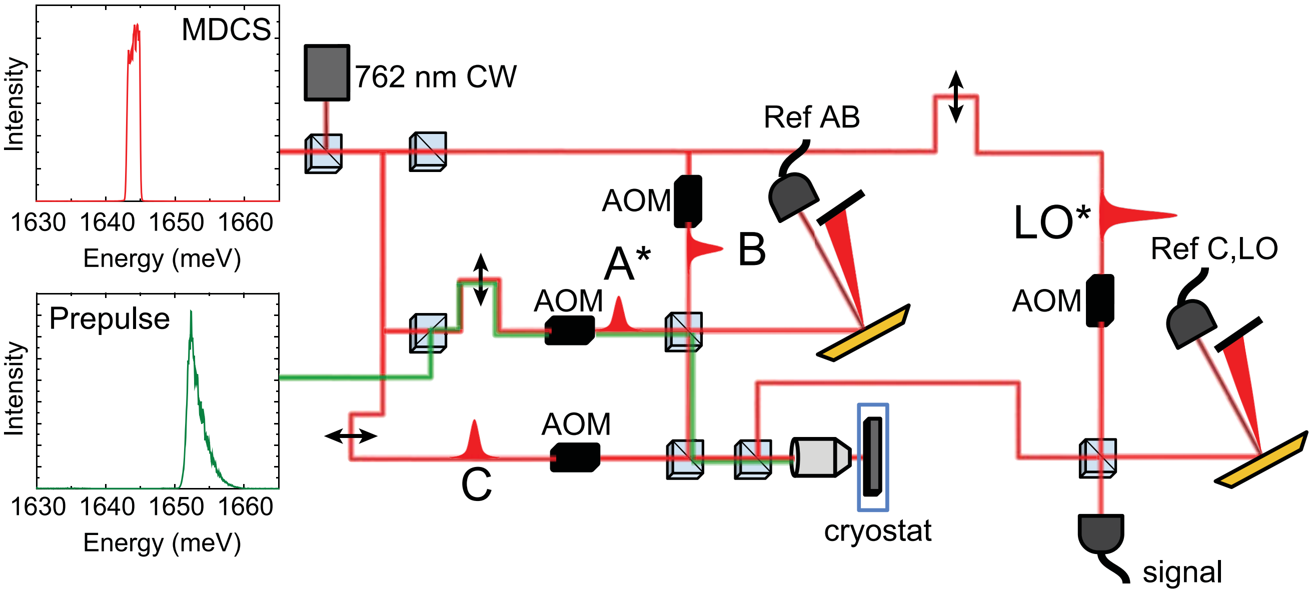


FIG. 1. Multidimensional coherent spectroscopy (MDCS) is used to probe interactions in the sample. The MDCS pulses are spectrally narrowed, plotted in the top inset, to resonantly excite the quantum dots states (QDs). These interactions are measured as a function of prepulse power, where the prepulse is spectrally narrowed to excite only the quasi-continuum quantum well states, plotted in the bottom inset. Acousto-optic modulators (AOMs) are used to frequency tag the MDCS beams A*, B, C, and LO*. A continuous-wave (CW) laser copropagates the MDCS beams to sample phase fluctuations in each arm. Gratings are used to separate the CW from the pulses on the reference detectors.

In Fig. 1, the beams are labelled A*, B, C, and LO* (for local oscillator) which are frequency shifted by $\omega_A$, $\omega_B$, $\omega_C$, and $\omega_{LO}$ respectively. Stars on the label indicate pulse conjugation. With these conjugates, the corresponding four-wave-mixing signal is tagged with $\omega_{FWM} = \omega_B - \omega_A + \omega_C - \omega_{LO}$. The phase corrected signal is generated using the interfered reference beams. The frequency detected on the reference detectors are $\omega_B - \omega_A$ and $\omega_C - \omega_{LO}$.

The pulse ordering A*-B-C-LO* corresponds to a single-quantum rephasing spectrum. One can simulteously measure the non-rephasing single-quantum spectrum by lock-in detecting at the frequency of sequence A-B*-C-LO*. In order to measure a double-quantum spectrum, the pulse order is changed to B-C-A*-LO* such that a double coherence evolves between C and A*.

## SINGLE-QUANTUM MDCS RESULTS

We simultaneously measure rephasing and non-rephasing single-quantum spectra using separate lock-in channels. We find that the single-quantum signals, shown in Figure 2, are also somewhat enhanced by prepulse excitation of the quantum well states. We also measure filling of the lower energy states as the peak of the nonlinear signal shifts towards higher energy quantum dots (QDs).

An interesting difference between the rephasing and non-rephasing sequences is also realized in this case of isolating individual QDs with a Gaussian beam. The spatial isolation of QDs by a tight focus, as opposed to a mask over the sample, offers the freedom to spatially scan over the sample. Unfortunately it leads to an inhomogeneous excitation of the QDs. Therefore, the strongest contributors to the signal are those QDs that are located near the spatial center of the beam. There are many more QDs near the edge of the beam that contribute to a background signal in our measurements. This is particularly noticeable for signals created by the rephasing pulse sequence in which all the weakly excited QDs constructively interfere to create a photon echo. Though the strongly excited QDs still dominate the signal, in a rephasing spectrum they sit on top of a background along the diagonal of weakly excited QDs, shown in Fig. 2(a)-(d). In the non-rephasing spectra, shown in Fig. 2(e)-(h) the strongly excited dots are more emphasized as many of the background excitations dephase each other.

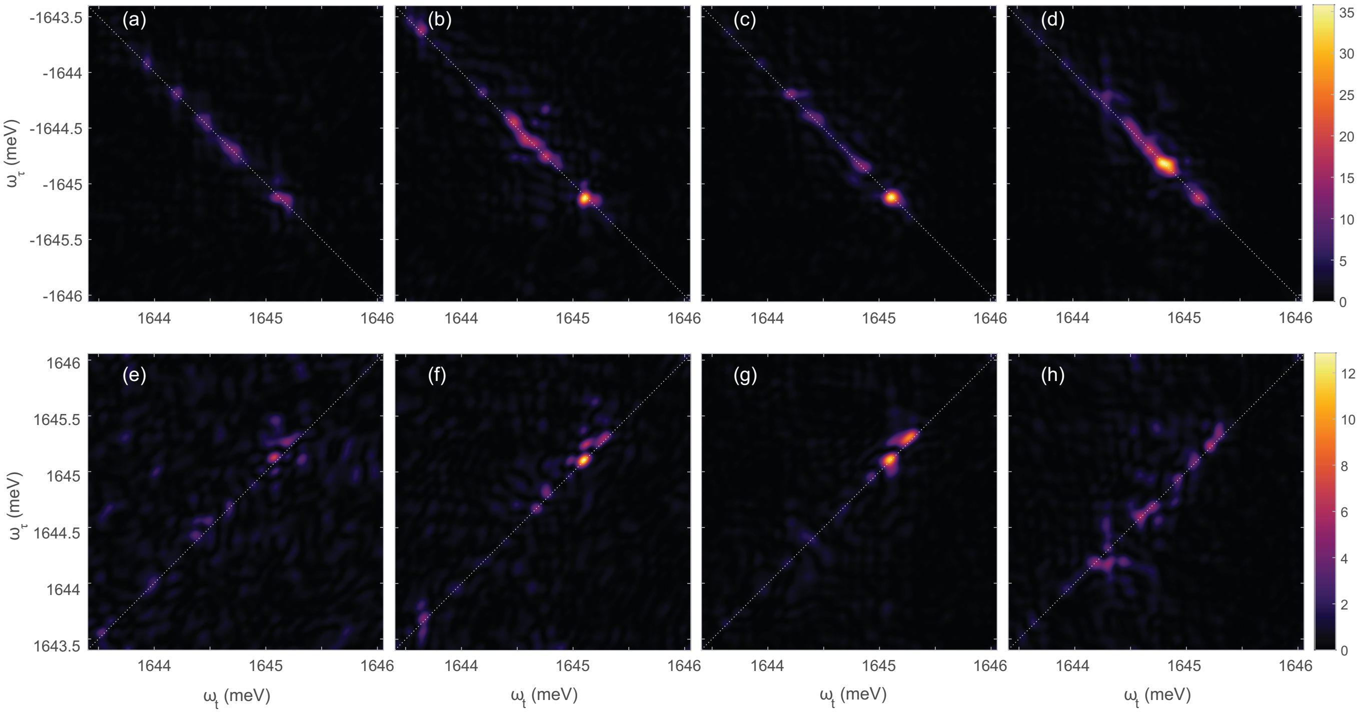


FIG. 2. Single-quantum spectra are also enhanced by prepulse excitatation. (a) is the rephasing spectrum with no prepulse excitation that is plotted in the paper. The other figures on the top row are rephasing spectra measured with prepulse powers of (b) 500, (c) 1500, and (d) 4000 photons per pulse. (e)-(h) are the corresponding non-rephasing spectra. The complete dephasing of the non-rephasing signal with high prepulse excitation is expected, while the increased rephasing signal strength can be attributed to the enhancement of the weakly excited background excitations.

## EVIDENCE THAT CONTINUUM COUPLED QDS ARE SPATIALLY DISTINCT

In a single-quantum measurement, off-diagonal features result from biexciton excitation and interexciton coupling. The biexciton states can be clearly identified by their binding energy shift from the absorption resonance, and all other features result from coupling of spatially distinct exciton resonances [5]. Single-quantum measurements are sensitive to all the interactions that a double-quantum measurement can measure (and more), and therefore the coupling features we measure with a double-quantum measurement will also only result from spatially distinct resonances.

To further support the statement that the prepulse is enhancing coupling between spatially distinct QD resonances, we measure a coupling feature at a different spot on the sample. These data are plotted in Fig. 3. In Fig. 3(a) and (b) we plot double-quantum spectra for a 0 and 500 photon prepulse, respectively. This demonstrates that these resonances respond to the continuum prepulse as discussed in the text. In Fig. 3(c) we plot a single-quantum rephasing measurement of the same position on the sample with dotted lines indicating the locations of the coupled resonances. We move the sample less than a spot diameter and measure the single-quantum spectrum of the new spot, plotted in Fig. 3(d). In the new spot one feature is enhanced while the other is suppressed, indicating that the two signals are emitted from different locations.

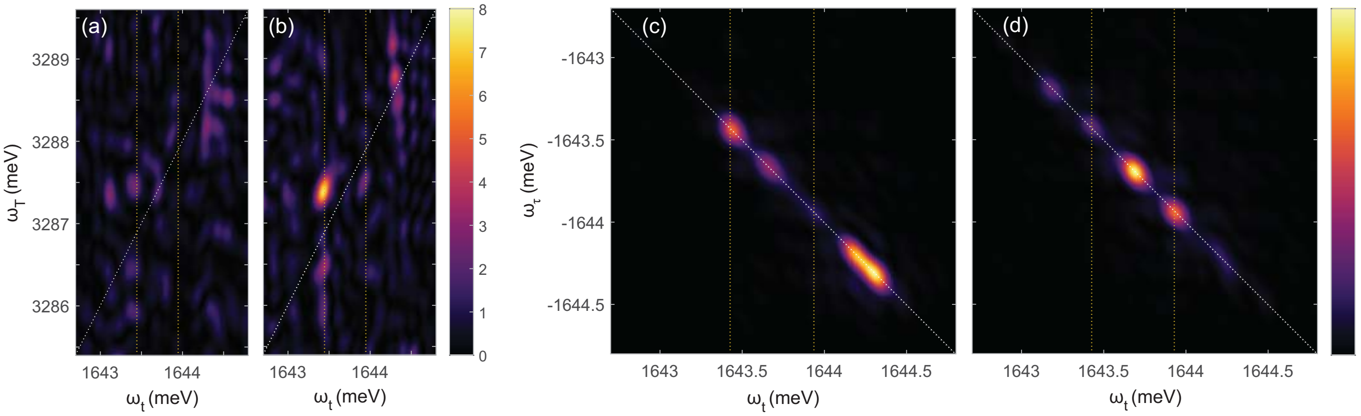


FIG. 3. We measure an enhanced coupling of two QDs using a prepulse and verify that the two QDs are spatially distinct. We plot double-quantum spectra of a spot on the sample in which we measure a coupling of QDs located at energies indicated by the vertical dotted lines using (a) no prepulse and (b) a 500 photon/pulse prepulse. In (c) we plot a measurement of the single-quantum spectrum at this spot on the sample. In (d) we measure the single-quantum spectrum of a spot spatially shifted less than a spot size away. We see the same resonances in (c) and (d), but the relative intensity of the resonances has changed as the lower energy QD is less efficiently measured by the new spot and the higher energy QD is more efficiently measured by the new spot.

## SAMPLE DESCRIPTION

Interfacial QDs are formed by width fluctuations of a GaAs quantum well [6–8]. The well is epitaxially grown with a nominal width of 15 monolayers, or 4.2 nm. The 35 nm barriers are made of $Al_{0.3}Ga_{0.7}As$. The growth of the top barrier is delayed by tens of seconds to give monolayer width fluctuations of the quantum well time to coalesce into islands. These islands, with a width of 16 monolayers, form the interfacial quantum dots, which are bound by 10 meV. The QDs cover approximately 2% of sample area and each have a size of approximately 36 nm [9].

## MODEL OF INTERACTIONS

QDs can generally be simulated as a simple two-level system. We add an additional weak coupling between two QDs in order to simulate the double-quantum spectra, which results in the energy-level scheme of a diamond configuration plotted in Fig. 4. The single excited states, $|e_1\rangle$ and $|e_2\rangle$, are located at 1644.19 meV and 1645.09 meV above the ground state. The doubly excited state is located at 3289.28 meV above the ground state with additional shifting and/or dephasing added as the source of the interaction signal. Since experimentally all of these energies are measured with respect to the evolution of a continuous-wave laser at 1627.5 meV, we also perform our simulations in this rotating

frame. In Fig. 5 we plot the response of each many-body effect on the real part of the simulated system, and we demonstrate how we can uniquely identify that the doubly excited state is shifted or dephased with respect to the sum of single excited states using double-quantum multidimensional spectroscopy.

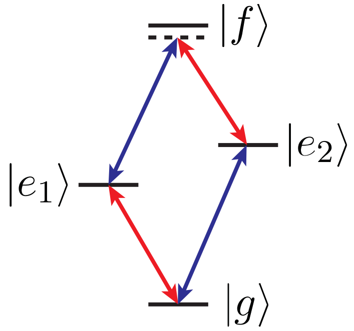


FIG. 4. The diamond configuration energy level diagram is used to model two coupled QDs with singly excited energy states $|e_1\rangle$ and $|e_2\rangle$. The doubly excited level is labeled $|f\rangle$ with the dotted line indicating that this level is either shifted or dephased from the non-interacting doubly excited level.

In Fig. 5, the phase of the signal resulting from a small (with respect to the linewidth of the resonance) excitation induced shift (EIS) of the double excited state is $\pm\pi/2$ from a signal resulting from purely excitation induced dephasing (EID) depending on whether the shift is blue or red. Any possible phase of the double quantum signal can therefore be determined by a combination of these effects. There is also an overall phase of the signal at the resonance which is uniquely determined by its double-quantum energy and the fixed $\tau$ delay at which the measurement is performed. This phase results from the evolution of the resonances during $\tau$, which is the lower energy state in half of the terms and the higher energy state in the other half with an equal oscillator strength for both. The overall phase, $\phi$, for any interaction resonance in a double quantum spectrum that can be modeled using coupled two-level systems is $-(\omega_1 + \omega_2)/\hbar \times \tau = -\omega_T/\hbar \times \tau$. If $\tau$ is set to 0 in the experiment, one can read off the phase of the interaction signal from the plot to determine EID (0), red EIS ($+\pi/2$), or blue EIS ($-\pi/2$). We typically set $\tau$ to a small finite value, however, to guarantee a correct pulse ordering in time. For the coupling resonance shown in the main text we calculate $\phi = -1.82$ rad. The phase of the signal in the experimental data is $-0.18 \pm 0.19$ rad, corresponding to an almost exactly $+\pi/2$ phase shift.

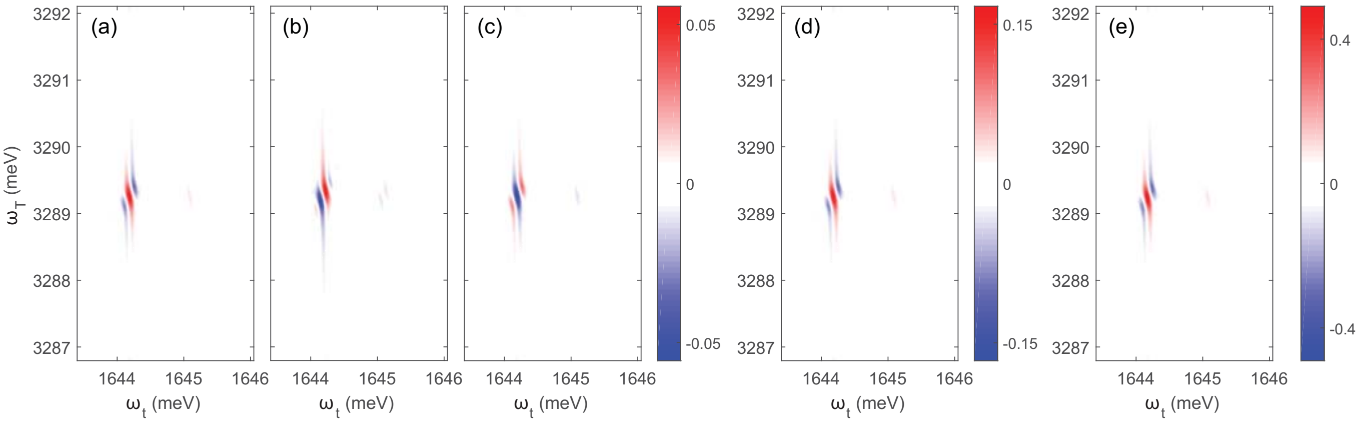


FIG. 5. We plot simulations of a double quantum signal resulting from a small (a) excitation induced shift of -0.003 meV, (b) excitation induced dephasing of 0.003 meV, and (c) excitation induced shift of +0.003 meV. We also show that as the magnitude of the excitation induced shift is increased, but still below the 0.05 meV linewidth, the general shape of the feature is unaffected. For (d) a shift of -0.009 meV and (e) a shift of -0.027 meV, the amplitude of the signal increases, but the phase does not.

Simulation of the diamond level structure requires the response function of all possible third-order nonlinear terms be considered. These response functions can be diagramatically represented with double-sided Feynman diagrams [10, 11]. In Fig. 6 we show have the diagram corresponding to terms for which the sample is initialized in the ground state. There are four equivalent diagrams in which the first absorption is from $|g\rangle$ into the $|e_2\rangle$ state. Since we fix the

$\tau$ delay, we do not resolve this. One can see by looking at these double-sided Feynman diagrams that excited state emission diagrams 1a and 2a have an opposite sign of the excited state absorption diagrams 1b and 2b. Also, without any interaction induced effects between $|e_1\rangle$ and $|e_2\rangle$, the emission energy of diagrams 1a and 1b (2a and 2b) is the same. Therefore, one can only measure a double-quantum signal if the emission energy from the doubly excited $|f\rangle$ to $|e_2\rangle$ differs from $|e_1\rangle$ to $|g\rangle$. This can only result from an interaction induced shift or dephasing of the doubly excited state [11].

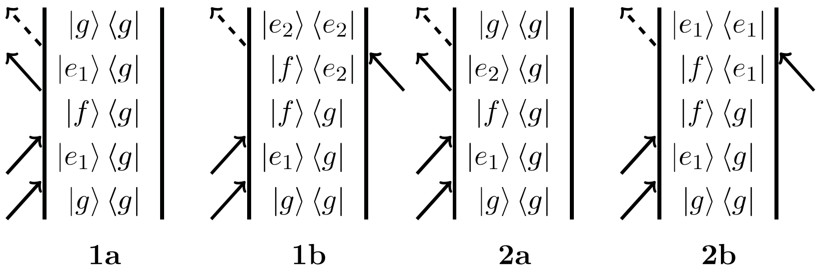


FIG. 6. These are double-sided Feynman diagrams corresponding to excitation of a double-quantum signal in the diamond configuration energy-level structure. These are all initialized in the ground state with the first excitation into the first excited state $|e_1\rangle$(there are four more equivalent diagrams first excited into $|e_2\rangle$). 1a and 1b both emit at the frequency corresponding to $|e_1\rangle$ and have opposite signs. A signal is emitted because there is some energy shift or dephasing of the double excited state $|f\rangle$ that is due to interaction between the two coherently excited states. 2a and 2b both emit at the $|e_2\rangle$ frequency and also have opposite signs.

In Fig. 7 we plot diagrams in which the prepulse has unintentionally excited an incoherent population in the localized states. We show diagrams for a singly excited population state and doubly excited population. Diagrams 1c-f give an identical lineshape to diagrams 1a and 1b, except that for the same emission energies they have an opposite sign. There are also twice as many diagrams for the prepulse excitation into the single excited state. For initial excitation of both involved quauntum dots, the sign is flipped again for constructive interference with the ground-state-initialized diagrams. Since $|\langle e_1 \,|\, e_1\rangle|^2 < 0.5$, these diagrams will not completely cancel. Thus measurements of the signal phase can be used to uniquely determine the relative energy shift and dephasing of the excited state.

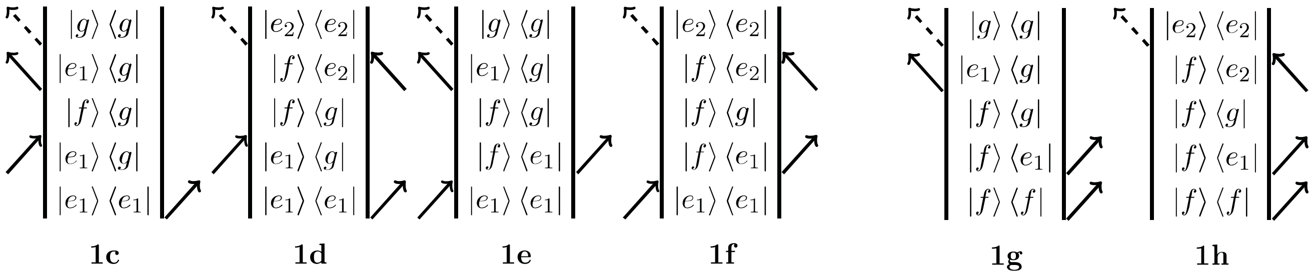


FIG. 7. Though the prepulse is resonant with the quasi-continuum states, some of those will relax into localized states prior to measurement by coherent spectroscopy. We must therefore consider initialization into the singly (1a-d) and doubly (1e-f) excited population states. The shapes of these response functions actually all look the same as the ground state diagrams. The signs of the singly excited states are all opposite, however, and therefore degrade the magnitude of the double quantum signal without distorting the phase. Here we only plot a fourth of the total number of diagrams, leaving out nearly equivalent diagrams and those with emission at the $|e_2\rangle$ frequency.

* cundiff@umich.edu

[1] G. Nardin, Semiconductor Science and Technology **31**, 023001 (2016).
[2] S. T. Cundiff and S. Mukamel, Phys. Today **66**, 44 (2013).
[3] P. F. Tekavec, G. A. Lott, and A. H. Marcus, The Journal of Chemical Physics **127**, 214307 (2007).
[4] G. Nardin, T. M. Autry, K. L. Silverman, and S. T. Cundiff, Opt. Express **21**, 28617 (2013).
[5] J. Kasprzak and W. Langbein, J. Opt. Soc. Am. B **29**, 1766 (2012).
[6] D. Gammon, E. S. Snow, B. V. Shanabrook, D. S. Katzer, and D. Park, Phys. Rev. Lett. **76**, 3005 (1996).

[7] D. Gammon, E. S. Snow, B. V. Shanabrook, D. S. Katzer, and D. Park, Science **273**, 87 (1996).
[8] H. Castella and J. W. Wilkins, Phys. Rev. B **58**, 16186 (1998).
[9] G. Moody, M. E. Siemens, A. D. Bristow, X. Dai, D. Karaiskaj, A. S. Bracker, D. Gammon, and S. T. Cundiff, Phys. Rev. B **83**, 115324 (2011).
[10] P. Hamm and M. Zanni, *Concepts and Methods of 2D Infrared Spectroscopy* (Cambridge University Press, 2011).
[11] L. Yang and S. Mukamel, Phys. Rev. Lett. **100**, 057402 (2008).
